# Supplementary material for: Flexible Exoskeleton Control Based on Binding Alignment Strategy and Full-arm Coordination Mechanism
Source: arXiv:2503.01338 source file (2025-03-03)
Supplement: Supplementary file 1 [file supplementary_material.pdf]

# Supplementary Material

## A. Force interaction analysis at a single binding point.

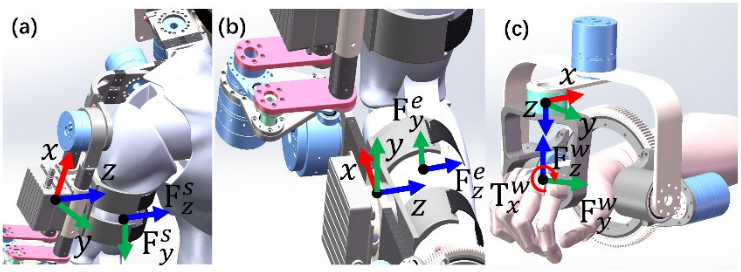


Fig. 1: The schematic diagram of the interaction forces between the exoskeleton and the human at the binding points at ideal state. The ideal state refers to: the exoskeleton being fully compatible with the human upper limbs, with no deviation in joint movements, no offset at the positions of the binding points, the user interacting with the exoskeleton with force applied at the center of binding attachments, and the force measured by force sensors reflecting the interaction force at that center (directly indicating the operator's movement intent). (a) is for the upper arm, (b) is for the forearm, and (c) is for the hand.

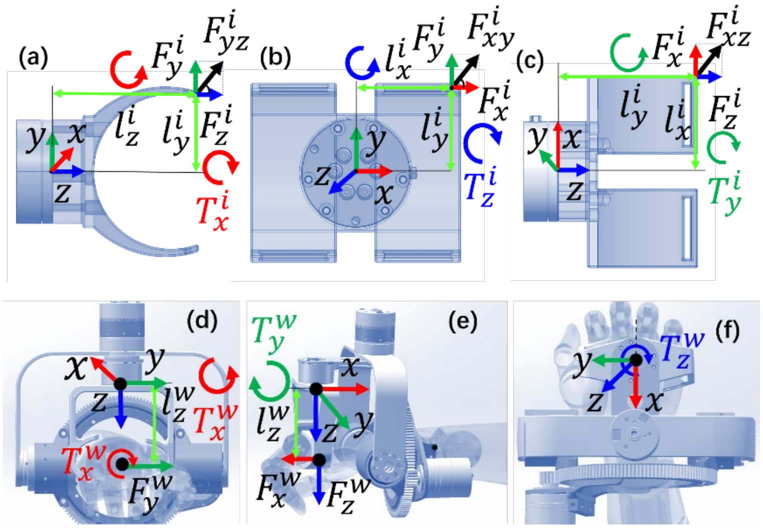


Fig. 2: (a-c) and (d-f) are schematic diagrams analyzing force sensors that measure general interaction forces at the upper arm/forearm and at the hand connection points. (a) and (d) are from the front view of the shoulder/elbow and hand binding attachment, while (b) and (e) are from the side view, and (c) and (f) are from the top view. In actual situations, the contact forces between the human arm and the binding attachments do not always act at the center of the attachments; they often occur at the edge positions.

The actual interaction forces at the binding points are shown in Fig. 2. The interaction forces at the upper arm and forearm binding attachments are affected by the donning offset, as shown in Fig. 2 (a-c). In practice, the contact force between the user's arm and the exoskeleton typically acts at the edge of the binding attachment, rather than at its center. The interaction force at any contact

point can be decomposed along the force line direction of the F/T sensor, which can be resolved into $F_x^i$, $F_y^i$, $F_z^i$ components. Then, the force acting on the edge of the binding device will generate unnecessary torque on the F/T sensor:

$$T_x^i = F_z^i l_y^i - F_y^i l_z^i, T_y^i = F_x^i l_z^i - F_z^i l_x^i, T_z^i = F_y^i l_x^i - F_x^i l_y^i. \quad (1)$$

$l_x^i$, $l_y^i$ and $l_z^i$ represent the distance from the edge contact point to the force sensor's center measurement point in the x, y, and z directions respectively. Regarding the bindings on UA and FA, unlike the ideal force state depicted in Fig. 1, there are additional components $F_x^i$, $T_x^i$, $T_y^i$, $T_z^i$ in Fig. 2 (a-c) generated in general motion. These additional components are influenced by the ideal force components $F_y^i$ and $F_z^i$.

Regarding the interaction forces at the hand attachment (Fig. 2 (d-f)), due to the limited design space of the exoskeleton hand, the sensors are installed far from the hand and the wrist joint. Therefore, disturbances occur when interaction forces are measured using the F/T sensors. For example, as illustrated in Fig.2(d), when the user wants to perform the wrist pronation/supination (Wr.Pr/Su), the user's hand will generate $T_y^w$, and when the user wants to perform the wrist ulnar/radial deviation (Wr.Ud/Rd), the user's hand will generate $F_y^w$ at the force sensor above the hand. However, this lateral force $F_y^w$ will also create a torque in the x-direction, $T_x^w = F_y^w l_y^w$, which will influence the movement of Wr.Pr/Su.

As shown in Fig. 2 (e), when the user wears the hand binding device and applies $F_z^w$ to drive the pitch motion of the wrist, it is inevitable that the force in the x-direction $F_x^w$ will be generated, which in turn will generate a torque $T_y^w$. Then, $T_y^w$ influences the pitch movement using the traditional control method based on statics. Fig. 2 (f) shows the disturbance torque $T_z^w$ due to the hand attachment not being entirely suitable for the user's hand-wearing. Higher torque values of $T_z^w$ signifies poorer hand conformity to the binding point during movement. This conformity can be improved by controlling the movement of the yaw joint, but the action is coupled with the active movement of Wr.Ud/Rd.

In summary, for the force interaction at a single binding point, additional components ($F_x^i$, $T_x^i$, $T_y^i$, $T_z^i$ in UA and FA, $F_x^w$, $T_y^w$, $T_z^w$ in HA) will inevitably arise. We expect to utilize some of these components to reduce the donning disturbance caused by the binding deviation in our control method proposed in **"the submitted manuscript"**.

## B. Calculation of the shoulder angle and the elbow angle

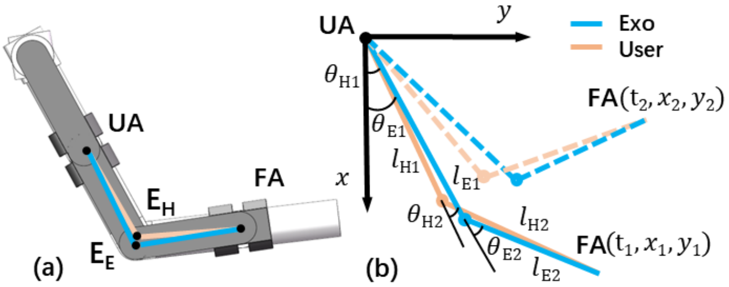


Fig. 3: (a) is the simplified model diagram illustrating mismatched sizes for wearing the exoskeleton on the user's upper arm and forearm. It is similar to two linked rods moving together in a sleeve. The model is further simplified to the rod model in (b). When the upper arm and forearm move together, there is a misalignment at the binding point between the upper arm and forearm rods of the user and the exoskeleton.

According to the cosine theorem,

$$\theta_{H1} = \text{acos}\frac{x}{\sqrt{x^2+y^2}} - \text{acos}\frac{x^2+y^2+{l_{H1}}^2-{l_{H2}}^2}{2l_{H1}\sqrt{x^2+y^2}},$$

$$\theta_{E1} = \text{acos}\frac{x}{\sqrt{x^2+y^2}} - \text{acos}\frac{x^2+y^2+{l_{E1}}^2-{l_{E2}}^2}{2l_{E1}\sqrt{x^2+y^2}}.$$

$\theta_{H1}$ and $\theta_{E1}$ represent the shoulder angle of the human and the exoskeleton.

$$\theta_{H2} = \pi - \text{acos}\frac{{l_{H1}}^2+{l_{H2}}^2-(x^2+y^2)}{2l_{H1}l_{H2}}$$

$$\theta_{E2} = \pi - \text{acos}\frac{{l_{E1}}^2+{l_{E2}}^2-(x^2+y^2)}{2l_{E1}l_{E2}}$$

where $\theta_{H2}$ and $\theta_{E2}$ represent the elbow angle of the human and the exoskeleton. $x, y$ are the coordinates of point FA in Fig. 3.

## C. Jacobian Matrix in the kinematics of the exoskeleton.

Regarding the binding alignment strategy, the Jacobian matrix for each binding point ${\boldsymbol{J}_{SC2}^{UA}}^{\mathrm{T}}$ , ${\boldsymbol{J}_{EL1}^{FA}}^{\mathrm{T}}$, ${\boldsymbol{J}_{WR1}^{HA}}^{\mathrm{T}}$ is as shown in the following formula:

$${\boldsymbol{J}_{SC2}^{UA}}^{\mathrm{T}} = \begin{bmatrix} a_2S_4 - d_3C_4S_3 & a_2C_4 - a_uS_3 + d_3S_3S_4 & C_3(d_3 - a_uS_4) & C_3C_4 & -C_3S_4 & S_3 \\ 0 & 0 & a_uC_4 & S_4 & C_4 & 0 \\ 0 & -a_u & 0 & 0 & 0 & 1 \end{bmatrix},$$

$${\boldsymbol{J}_{EL1}^{FA}}^{\mathrm{T}} = \begin{bmatrix} 0 & 0 & a_eC_6 & -S_6 & -C_6 & 0 \\ 0 & a_e & 0 & 0 & 0 & 1 \end{bmatrix},$$

$${\boldsymbol{J}_{WR1}^{HA}}^{\mathrm{T}} = \begin{bmatrix} 0 & 0 & a_wS_8 & a_wC_8S_9 & C_8C_9 & -C_8S_9 \\ 0 & 0 & 0 & -a_wC_9 & S_9 & S_9 \\ 0 & 0 & a_w & 0 & 0 & 0 \end{bmatrix},$$

where $S_i$ and $C_i$ represent the $\sin(\theta_i)$ and $\cos(\theta_i)$ respectively of the i-th joint, $a_2$, $d_3$, $a_u$, $a_e$, $a_w$ represent the offset parameters between link coordinate systems in the kinematics of the exoskeleton as show in **Fig. 2 of "the submitted manuscript"**. The definition of the coordinate systems of the links of the exoskeleton refers to "**TABLE VI in literature [1]**".

We obtain the coordinate transformation relationships between the links and then calculate the various kinematic models $\boldsymbol{T}_{SC2}^{UA}$, $\boldsymbol{T}_{EL1}^{FA}$ and $\boldsymbol{T}_{WR1}^{HA}$ based on the definition of the coordinate systems of each link, as referenced in **literature [2]** and **literature [3]**.

Regarding the full-arm coordination mechanism, the Jacobian matrix $\boldsymbol{J}_{SC1}^{UA}$,$\boldsymbol{J}_{SC1}^{FA}$ and $\boldsymbol{J}_{SC1}^{HA}$ for each binding point for the full-arm coordination control can be calculated using the method described above. Among them, $\boldsymbol{T}_{SC1}^{UA}$, $\boldsymbol{T}_{SC1}^{FA}$and $\boldsymbol{T}_{SC1}^{HA}$ can be obtain by the following formula:

$$\boldsymbol{T}_{SC1}^{UA} = \boldsymbol{A}_{SC1}^{SC2}\boldsymbol{T}_{SC2}^{UA}$$

$$\boldsymbol{T}_{SC1}^{FA} = \boldsymbol{T}_{SC1}^{UA}\boldsymbol{A}_{UA}^{EL1}\boldsymbol{T}_{EL1}^{FA}$$

$$\boldsymbol{T}_{SC1}^{HA} = \boldsymbol{T}_{SC1}^{FA}\boldsymbol{A}_{FA}^{WR1}\boldsymbol{T}_{WR1}^{HA}$$

$\boldsymbol{A}_{SC1}^{SC2}$ is the transformation matrix corresponding to joint SC1. $\boldsymbol{A}_{UA}^{EL1}$ and $\boldsymbol{A}_{FA}^{WR1}$ represent the transformation matrices from the first elbow joint to the upper arm binding point and from the first wrist joint to the forearm binding point, respectively. Both of them only have translation transformations, and thus, they are all constant matrices.


[1] C. Cheng et al., "Efficient and Precise Homo-Hetero Teleoperation Based on an Optimized Upper Limb Exoskeleton," in *IEEE/ASME Transactions on Mechatronics*, doi: 10.1109/TMECH.2024.3479873.

[2] Paul, Richard P., "Robot manipulators : mathematics, programming, and control ," in *The MIT Press*, 1981.

[3] Saeed B. Niku., "Introduction to Robotics: Analysis, Control, Applications, 2nd Edition ," in John Wiley & Sons, Inc., 2011.

## D. The parameters of the dynamics and the control system of the exoskeleton.

TABLE. I: The inertia and gravity parameters of the exoskeleton.

| Link | $I_{xx}$ (g·mm²) | $I_{yy}$ (g·mm²) | $I_{zz}$ (g·mm²) | $I_{xy}$ (g·mm²) | $I_{xz}$ (g·mm²) | $I_{yz}$ (g·mm²) | **m** (g) | **x** (mm) | **y** (mm) | **z** (mm) |
|---|---|---|---|---|---|---|---|---|---|---|
| #1 | 827503.80 | 998784.44 | 698284.09 | -625.47 | 721.11 | -2821.02, | 739.56 | -6.65 | 0.07 | -20.29 |
| #2 | 6614490.13 | 8839106.31 | 2736457.63 | 3098.93 | 1242372.67 | 250.53 | 891.23 | 25.87 | 0.03 | 79.57 |
| #3 | 2754993.58 | 1163318.65 | 1878724.16 | 6085.93 | 10000.13 | 828537.24 | 295.34 | -0.50 | -66.00 | -51.50 |
| #4 | 46471391.21 | 25548403.81 | 23128759.60 | -4120.00 | -30960.67 | 17866672.58 | 3226.86 | -0.10 | 107.5 | 88.13 |
| #5 | 19028898.11 | 18250653.74 | 2603927.94 | 197793.06 | 1609462.27 | 3560146.79 | 1080.76 | -7.99 | -23.01 | -110.17 |
| #6 | 29009300.02 | 26532590.34 | 3660469.61 | -25009.93 | -47864.72 | 5268052.60 | 832.18 | -0.34 | 45.10 | 150.15 |
| #7 | 1991830.07 | 2078498.76 | 352414.43 | 42.07 | 362.05 | -16436.87 | 439.99 | 0 | 6.73 | -1.68 |
| #8 | 3999782.87 | 2922055.28 | 1138186.71 | -56.65 | -1080.74 | -3548.93 | 309.94 | 0.02 | 0.74 | 87.75 |
| #9 | 770470.53 | 706416.01 | 152856.67 | 240.39 | -66070.63 | 663.38 | 161.96 | -4.31 | 0.11 | 49.55 |

$I_{xx}$, $I_{yy}$, $I_{zz}$, $I_{xy}$, $I_{xz}$ and $I_{yz}$ are the parameters of moment of inertia. **m** denotes the mass of each link. **x, y, z** represent the coordinates of the mass centroid.

TABLE. II: The friction parameters of the exoskeleton.

| Link | #1 | #2 | #3 | #4 | #5 | #6 | #7 | #8 | #9 |
|---|---|---|---|---|---|---|---|---|---|
| $f_s$ | 460 | 440 | 450 | 450 | 220 | 200 | 50 | 50 | 50 |
| $f_c$ | 560 | 530 | 530 | 540 | 280 | 260 | 100 | 100 | 100 |
| $v_c$ (rad/s) | 1.75 | 1.71 | 1.77 | 1.73 | 1.65 | 1.68 | 1.54 | 1.56 | 1.55 |
| $a$ | 500 | 400 | 600 | 500 | 200 | 300 | 100 | 100 | 100 |

TABLE. III: The parameters in the binding alignment strategy (BAS).

| $F^s_{ymax}$ | $F^s_{zmax}$ | $F^e_{ymax}$ | $F^e_{zmax}$ | $F^w_{ymax}$ | $F^w_{zmax}$ |
|---|---|---|---|---|---|
| 16N | 12N | 7N | 5N | 2.7N | 3.2N |

TABLE. IV: The parameters in the full-arm coordination mechanism (FCM).

| $F^s_{y\_th}$ | $F^s_{z\_th}$ | $F^e_{y\_th}$ | $F^e_{z\_th}$ | $F^w_{y\_th}$ | $F^w_{z\_th}$ |
|---|---|---|---|---|---|
| 0.6N | 0.5N | 0.45N | 0.35N | 0.2N | 0.2N |
| $F^s_{y\_c}$ | $F^s_{z\_c}$ | $F^e_{y\_c}$ | $F^e_{z\_c}$ | $F^w_{y\_c}$ | $F^w_{z\_c}$ |
| 5N | 5N | 3.5N | 3N | 1.5N | 1.7N |

## E. Detailed numerical results of the experiment of *Adaptability*.

TABLE. V: Average Torque error (assistant component) at the binding points during *Adaptability* experiment.

| AC | Method | 0.5rad/s ATV | AIT | 1.0rad/s ATV | AIT | 1.5rad/s ATV | AIT | 2.0rad/s ATV | AIT | 2.5rad/s ATV | AIT | 3.0rad/s ATV | AIT | 3.5rad/s ATV | TAIT |
|---|---|---|---|---|---|---|---|---|---|---|---|---|---|---|---|
| $T_z^e$ | FF$_D$ | **0.169** | **-0.086** | **0.083** | 0.718 | -0.801 | 1.137 | -1.938 | **0.100** | -2.038 | **-0.206** | -1.832 | **0.106** | -1.938 | 2.107 |
| | FF$_U$ | 0.958 | -0.082 | 0.876 | 0.090 | 0.966 | 0.563 | 1.529 | **-0.191** | 1.338 | 0.376 | 1.714 | 0.090 | 1.804 | 0.846 |
| | VMC$_D$ | 0.122 | 0.121 | -0.243 | 0.443 | -0.686 | 0.458 | -1.144 | 0.225 | -1.369 | -0.015 | -1.354 | 0.138 | -1.492 | 1.614 |
| | VMC$_U$ | 0.792 | **-0.119** | 0.673 | **0.015** | 0.688 | 0.277 | 0.965 | 0.226 | 1.191 | 0.355 | 1.546 | 0.116 | 1.662 | 0.869 |
| | BAS$_D$ | -0.023 | 0.119 | -0.142 | **0.202** | **-0.344** | **0.318** | **-0.662** | 0.306 | **-0.968** | 0.007 | **-0.975** | 0.126 | **-1.101** | **1.079** |
| | BAS$_U$ | **0.631** | -0.028 | **0.603** | 0.084 | **0.687** | **-0.052** | **0.635** | 0.416 | **1.051** | **0.165** | **1.216** | **-0.047** | **1.169** | **0.538** |
| $T_y^e$ | FF$_D$ | -0.334 | -0.138 | -0.196 | 0.186 | -0.382 | 0.297 | -0.679 | 0.076 | -0.755 | **0.105** | -0.860 | **0.094** | -0.954 | 0.604 |
| | FF$_U$ | 1.121 | -0.063 | 1.057 | -0.200 | 0.857 | 0.118 | 0.975 | **0.145** | 1.152 | 0.072 | 1.224 | 0.114 | 1.338 | 0.217 |
| | VMC$_D$ | -0.250 | -0.154 | -0.096 | 0.286 | -0.372 | 0.007 | -0.379 | -0.124 | -0.255 | 0.201 | -0.456 | 0.298 | -0.754 | 0.504 |
| | VMC$_U$ | 1.025 | **-0.090** | 0.935 | -0.178 | 0.757 | 0.023 | 0.780 | 0.243 | 1.023 | -0.199 | 0.824 | 0.214 | 1.038 | 0.013 |
| | BAS$_D$ | **-0.053** | **-0.157** | **0.104** | **0.078** | **-0.182** | **-0.003** | **-0.179** | **-0.031** | **-0.148** | 0.108 | **-0.256** | 0.098 | **-0.354** | **0.304** |
| | BAS$_U$ | **0.835** | -0.077 | **0.758** | **-0.201** | **0.557** | **-0.087** | **0.470** | 0.341 | **0.811** | **-0.187** | **0.624** | **0.014** | **0.638** | **-0.197** |
| $T_z^s$ | FF$_D$ | -0.287 | -0.1169 | -0.170 | **-0.060** | **-0.110** | 0.043 | -0.153 | 0.119 | -0.272 | **0.030** | -0.302 | 0.386 | -0.688 | 0.401 |
| | FF$_U$ | 0.721 | **0.0702** | 0.791 | 0.104 | 0.895 | -0.026 | 0.869 | **-0.052** | 0.817 | 0.014 | 0.831 | **-0.010** | 0.821 | **0.100** |
| | VMC$_D$ | -0.227 | -0.1196 | -0.107 | 0.048 | -0.155 | 0.019 | -0.174 | 0.008 | -0.182 | 0.070 | -0.252 | 0.236 | -0.488 | 0.261 |
| | VMC$_U$ | 0.521 | 0.2302 | 0.751 | 0.044 | 0.795 | **-0.126** | 0.669 | 0.118 | 0.787 | -0.156 | 0.631 | 0.102 | 0.733 | 0.212 |
| | BAS$_D$ | **-0.200** | **-0.1945** | **-0.006** | 0.104 | **-0.110** | **-0.022** | **0.088** | 0.044 | **-0.132** | 0.078 | **-0.210** | **0.077** | **-0.287** | **0.086** |
| | BAS$_U$ | **0.182** | 0.479 | **0.661** | **-0.062** | **0.589** | 0.002 | **0.591** | **0.155** | **0.746** | **-0.222** | **0.524** | 0.114 | **0.638** | 0.456 |
| $T_y^s$ | FF$_D$ | -0.450 | **0.078** | -0.528 | -0.044 | -0.484 | 0.298 | -0.782 | 0.218 | -1.000 | 0.376 | -1.376 | 0.139 | -1.515 | 1.066 |
| | FF$_U$ | 0.510 | **0.079** | 0.589 | -0.059 | 0.530 | 0.092 | 0.622 | 0.499 | 1.119 | 0.161 | 1.280 | 0.193 | 1.473 | 0.963 |
| | VMC$_D$ | -0.319 | 0.152 | -0.471 | **-0.057** | -0.414 | 0.268 | -0.682 | 0.216 | -0.898 | 0.300 | -1.198 | 0.084 | -1.282 | 0.963 |
| | VMC$_U$ | 0.459 | 0.026 | 0.485 | **-0.069** | 0.416 | 0.300 | 0.716 | 0.203 | 0.919 | **0.129** | 1.048 | 0.199 | 1.247 | 0.788 |
| | BAS$_D$ | **-0.245** | 0.126 | **-0.371** | -0.041 | **-0.330** | **0.152** | **-0.482** | **0.116** | **-0.598** | **0.103** | **-0.701** | **0.181** | **-0.882** | **0.637** |
| | BAS$_U$ | **0.165** | 0.140 | **0.305** | 0.061 | **0.366** | **0.121** | **0.487** | **-0.168** | **0.319** | 0.153 | **0.472** | **-0.001** | **0.473** | **0.308** |
| $T_z^s + T_z^e$ | FF$_D$ | -1.957 | 0.591 | -2.548 | 1.013 | -3.561 | **0.2028** | -3.764 | 0.435 | -4.199 | **0.394** | -4.593 | **0.143** | -4.736 | 2.779 |
| | FF$_U$ | 2.282 | **0.226** | 2.508 | 0.997 | 3.505 | **0.073** | 3.578 | 0.930 | 4.508 | **0.212** | 4.720 | 0.559 | 5.279 | 2.997 |
| | VMC$_D$ | -2.023 | 0.133 | -2.176 | **0.252** | -2.428 | 0.936 | -3.364 | 0.510 | -3.874 | 0.521 | -4.395 | 0.083 | -4.478 | 2.455 |
| | VMC$_U$ | 2.067 | 0.269 | 2.336 | **0.236** | 2.572 | 0.659 | 3.231 | 0.577 | 3.808 | 0.426 | 4.234 | 0.477 | 4.711 | 2.644 |
| | BAS$_D$ | **-1.050** | **0.042** | **-1.092** | 0.329 | **-1.421** | 0.747 | **-2.168** | **0.259** | **-2.427** | 0.840 | **-3.267** | 0.233 | **-3.500** | **2.451** |
| | BAS$_U$ | **0.653** | 0.846 | **1.499** | 0.358 | **1.857** | 0.426 | **2.283** | **0.268** | **2.551** | 0.408 | **2.959** | **-0.139** | **2.820** | **2.167** |
| $T_y^s + T_y^e$ | FF$_D$ | -2.065 | **-0.432** | -1.633 | 0.785 | -2.418 | 1.020 | -3.438 | **0.451** | -3.889 | **0.504** | -4.393 | 0.143 | -4.536 | 2.471 |
| | FF$_U$ | 2.171 | **-0.452** | 1.719 | 0.618 | 2.337 | 1.321 | 3.658 | **0.368** | 4.026 | **0.293** | 4.319 | 0.544 | 4.863 | 2.692 |
| | VMC$_D$ | -1.503 | 0.252 | -1.755 | **0.399** | -2.154 | **0.726** | -2.880 | 0.861 | -3.741 | 0.533 | -4.274 | **0.023** | -4.297 | 2.795 |
| | VMC$_U$ | 1.437 | 0.554 | 1.991 | **0.321** | 2.312 | **0.493** | 2.805 | 0.981 | 3.786 | 0.347 | 4.133 | 0.478 | 4.611 | 3.174 |
| | BAS$_D$ | **-0.916** | -0.349 | **-0.577** | 0.712 | **-1.289** | 0.641 | **-1.930** | 0.524 | **-2.454** | 0.791 | **-3.245** | 0.058 | **-3.303** | **2.386** |
| | BAS$_U$ | **0.899** | -0.180 | **0.719** | 0.581 | **1.300** | 0.768 | **2.068** | 0.483 | **2.551** | 0.408 | **2.959** | **-0.383** | **2.576** | **1.677** |

The unit of speed (0.5~3.5) is rad/s. AC denotes assistant component i.e. the torque value corresponding to the interaction force at the binding point. ATV represents the average torque value of several times test results for the experiment at each set of speed. AIT represents absolute increase of the torque value between the two group of the speed for these experiments. TAIT represents the total absolute value of the torque increase from 0.5~3.5rad/s. The subscripts D and U represent the lower and upper limits, respectively.

This table represents the numerical data of the histogram in **Fig. 11 of "the submitted manuscript"**. The values highlighted in **red** indicate that the average torque error at this speed for deploying the algorithm is smaller than that of other algorithms, while the values in **bold** indicate whose AIT is relatively small. Based on the results of this table and **Fig. 11 of "the submitted manuscript"**, the BAS method we proposed has advantages both in terms of the average torque value and the total absolute value of the torque increase during the experiments from low speed to high speed. It indicates that our method can reduce the donning disturbance torque caused by binding deviation of the upper limb exoskeleton during movements.

# F. Other results of the experiment of *Speed*.

In **"the submitted manuscript"**, we only presented the curve of the linear speed of the end of the exoskeleton during the fast dynamic motion. Here, we add the curves of angular speed and each joint speed of the exoskeleton during the fast dynamic motion.

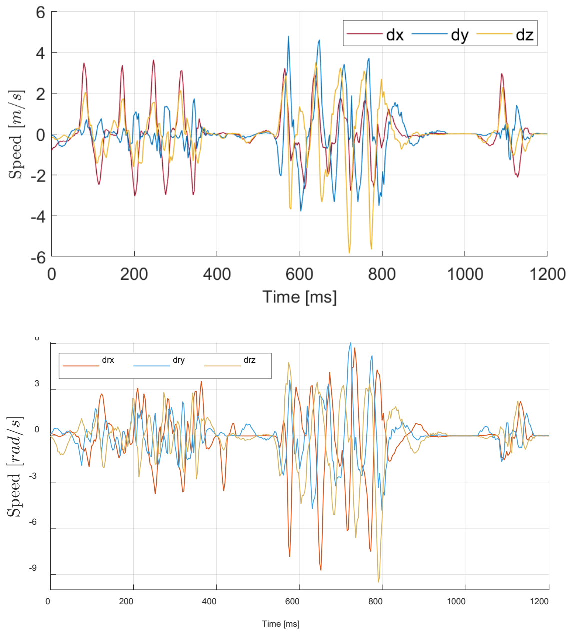


Fig. 4: Linear and angular speed of the end of the exoskeleton during the fast dynamic motion.

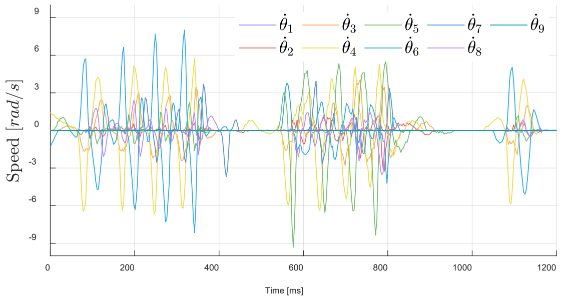


Fig 5: Each joint speed of the exoskeleton during the fast dynamic motion.

## G. Other results of the experiment of Fatigue with EMG.

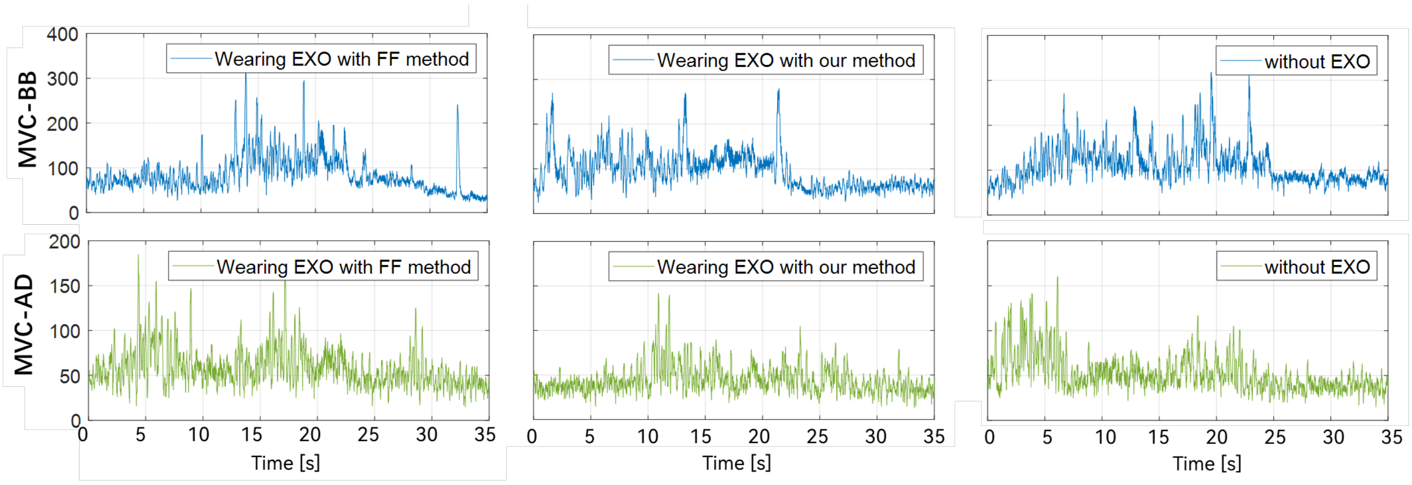


Fig 6: Muscle activation level (measured by EMG) comparison between with FF method (The feed-forward compensation with the traditional decoupling active force controller) and our method (BAS + FCM) during wearing the exoskeleton and without the exoskeleton. Bule curves represent muscle activation of voluntary contraction (MVC) biceps brachii (BB) and green curves represent that of anterior deltoid (AD).

This figure serves as a supplement to **Fig. 15 and TABLE VII in "the submitted manuscript"**, where we present data on muscle activation measured by electromyography (EMG) devices under four conditions in the fatigue experiment: (1) wearing the exoskeleton without control, (2) wearing the exoskeleton using the feed-forward compensation with the traditional decoupling active force controller (FF), (3) wearing the exoskeleton with our control method and (4) the user moves freely without wearing the exoskeleton. Our method requires less muscle strength when performing movements while wearing the exoskeleton, and the data curves are very similar to the situation where the user performs movements freely without wearing an exoskeleton.
